# Supplementary material for: Reaching the intrinsic performance limits of superconducting nanowire single-photon detectors up to 0.1 mm wide
Source: arXiv:2601.15971 source file (2026-07-23)
Supplement: Supplementary file 2 [file maina.pdf]

# Approaching the intrinsic performance limits of superconducting strip photon detectors up to 0.1 mm wide

Kristen M. Parzuchowski<sup>1,2\*†</sup>, Eli Mueller<sup>1,3†</sup>,  
Bakhrom G. Oripov<sup>1,2</sup>, Benedikt Hampel<sup>1,2</sup>,  
Ravin A. Chowdhury<sup>1,2</sup>, Sahil Patel<sup>4</sup>, Daniel Kuznesof<sup>5</sup>,  
Emma K. Batson<sup>1,6</sup>, Varun B. Verma<sup>1</sup>, Jason P. Allmaras<sup>4</sup>,  
Martin J. Stevens<sup>1</sup>, Alex Gurevich<sup>7</sup>, Adam N. McCaughan<sup>1,2</sup>

<sup>1\*</sup>National Institute of Standards and Technology, Boulder, CO, U.S.A.

<sup>2</sup>University of Colorado, Boulder, CO, U.S.A.

<sup>3</sup>University of Colorado, Denver, CO, U.S.A..

<sup>4</sup>Jet Propulsion Laboratory, California Institute of Technology,  
Pasadena, CA, U.S.A.

<sup>5</sup>University of Glasgow, Glasgow, U.K.

<sup>6</sup>Massachusetts Institute of Technology, Cambridge, MA, U.S.A.

<sup>7</sup>Department of Physics, Old Dominion University, Norfolk, VA, U.S.A.

\*Corresponding author(s). E-mail(s): [kristen.parzuchowski@nist.gov](mailto:kristen.parzuchowski@nist.gov);

Contributing authors: [eli.mueller@nist.gov](mailto:eli.mueller@nist.gov);

<sup>†</sup>These authors contributed equally to this work.

## Abstract

Superconducting nanowire single photon detectors have become an enabling technology for quantum optics owing to their high detection efficiency, picosecond timing precision, and low dark count rates. Yet even the best detectors fall short of their ultimate performance limits due to lithographic defects and current crowding at the wire edges which restrict device sizes and infrared sensitive detector widths below 100 nm. Here, we demonstrate for the first time detectors integrated with current rails which allow *in-situ tuning* to their ultimate performance limit by controllable reduction of current density at the wire edges. We report a 100  $\mu\text{m}$ -wide detector that achieves 100% internal detection efficiency

at 1550 nm, and a reduction in dark count rate by up to eight orders of magnitude. We also demonstrate a 20  $\mu\text{m}$ -wide detector with nearly 100% efficiency at 4  $\mu\text{m}$ . By overcoming the fundamental detector size limitations, this work establishes a new class of high-performance, ultra-wide superconducting strip photon detectors. Such devices will enable large-area, high efficiency detector arrays with infrared sensitivity and open new opportunities for applications ranging from diffuse correlation spectroscopy to deep space optical communication.

## 1 Introduction

Overcoming the fundamental size and performance limitation of superconducting strip photon detectors (SSPDs) is necessary to achieve large-area high efficiency SSPD arrays sensitive into the infrared light, which are critical for many emerging technologies ranging from diffuse correlation spectroscopy [?] to exoplanet transit spectroscopy [?]. Such detectors reach a nearly 100 % photon sensitivity in the range of bias currents  $I_i < I_s < I_{sw}$ , where the onset current  $I_i$  and the switching current  $I_{sw}$  are fractions of the depairing current  $I_d$  - the maximum current a superconducting film can carry. Boosting the performance of SSPD requires increasing the detection range  $I_{sw} - I_i$ , yet even in state-of-the-art SSPDs, the switching current rarely exceeds 70% of the depairing limit [?].

A key advantage of reaching higher  $I_{sw}/I_d$  ratio is the ability to overcome the trade-off between the maximum strip width and the minimum photon energy sensitivity. Typically, detecting lower energy photons requires decreasing strip width to maintain the same energy deposited per cross sectional area. As a result, extending high efficiency SSPD's into the mid infra red (MIR) region has typically required strip widths of less than 100 nm [?]. However, as the operating current of the strip  $I_s$  approaches  $I_d$ , the photon energy required to form a critical hotspot expanding across the strip decreases. As a result, the minimum detectable photon energy at  $0.7I_d \leq I_{sw} < I_d$  was predicted to be only weakly dependent on the strip width [?], which opens the opportunity of developing very sensitive wide SSPDs operating at  $I_s \approx I_d$ . In addition, increasing  $I_{sw}/I_d$  suppresses dark count rate which depends exponentially on the proximity of the operating current to  $I_{sw}$ .

There are two technological and geometrical issues that limit how close  $I_{sw}$  can approach  $I_d$  in wide strips. First, thin film strips inevitably have lithographic defects causing localized current crowding along the edges [?]. Second, the Meissner effect causes a non-uniform flow of sheet current density  $J(x)$  across the strip, with  $J(x)$  being lowest at the center and maximum at the edges. This non-uniformity increases with the strip width  $w$  and becomes detrimental for the SSPD performance as the width exceeds the magnetic Pearl length  $\Lambda_s$  [?]. These two effects decrease the energy barrier for entry of superconducting vortices in the strip, greatly increasing the dark count rate due to thermally-activated penetration of vortices from the edges at currents well below  $I_d$ . Here we show that this problem can be resolved by introducing a novel SSPD architecture which provides an inverted  $J(x)$  profile having a flat portion in the main photon-sensitive part of the strip and tunable narrow dips at the edges

which block penetration of vortices by deactivating the edge defects. As a result, the SSPD performance and the maximum switching current becomes only limited by the fundamental unbinding of vortex-antivortex pairs inside the strip. It is the vortex-antivortex unbinding which determines the ultimate performance limit of SSPD and a maximum  $I_{sw}$  which is always smaller than  $I_d$ . In this work we report achieving this performance limit on WSi SSPD of different widths up to 0.1 mm.

In our SSPD architecture  $J(x)$  in the strip *is tuned in situ* by two adjacent current-carrying superconducting "rails", as shown in Fig. 1(a). Here, the magnetic field of the rails counters the perpendicular component of the field of the SSPD that causes the current crowding at the edges. The rails result in a redistribution of the current density in the strip with controllable dips in  $J(x)$  at the edges. Figure 1(c) shows the evolution of  $J(x)$  calculated by solving the London equation for different rail currents  $I_r$  (see Appendix D for details). This SSPD-rail architecture not only eliminates the edge current crowding relative to that of a single strip without rails, but also allows in-situ tuning of  $J(x)$  at the edge by varying  $I_r$  to optimize the SSPD performance. This novel approach offers a principal opportunity to break the Pearl limit and develop high-performance SSPDs with  $w > \Lambda_s$ . For instance, Fig. D2(b) in Appendix D shows tunable  $J(x)$  profiles calculated for a strip that is 4 times larger than  $\Lambda_s$ .

We have implemented the SSPD-rail architecture with a variety of 3 nm thick WSi thin films of different widths integrated with adjacent niobium film rails. By tuning the rail current, we were able to reduce the dark count rate by more than 8 orders of magnitude in a 100  $\mu\text{m}$ -wide SSPD. In a 20  $\mu\text{m}$ -wide SSPD, we reached a nearly 100% internal detection efficiency of 4  $\mu\text{m}$  photons and lowered detector jitter by about 30%. The rails allowed us to recover a detection plateau at 1550 nm in a device that would otherwise not be photosensitive because of its low  $I_{sw}/I_d$  ratio. These significant improvements were made without compromising the photon detection efficiency across the SSPD. Moreover, tuning  $J(x)$  by rails enables us to reach the operational maximum of  $I_{sw}$  for any SSPD without knowledge of the exact value  $J_d$  and the extent of detrimental effect of edge defects. This work not only demonstrates in situ tuning of an SSPD to its ultimate performance limit but also establishes a pathway to scaling straight long SSPDs to widths exceeding the Pearl length.

## Results

Our SSPD were fabricated from 3 nm thick WSi films which had the superconducting transition temperature  $T_c \approx 3.1\text{K}$ , the London penetration depth  $\lambda_s \approx 950\text{ nm}$  at 1K, the Pearl length  $\Lambda_s = 2\lambda_s^2/d \approx 602\text{ }\mu\text{m}$  and the normal state resistivity  $\rho_n \approx 2.5\text{ }\mu\Omega\cdot\text{m}$  at  $T = T_c$ . Details of the film deposition in SSPD and the measurements of materials parameters are given in Methods and Appendix A. The depairing current  $I_d$  and the Pearl length were evaluated for each film by measuring a nonlinear kinetic inductance, as described in Appendix B. For the rails, we used 50 nm thick Nb films of widths ranging from xx to 100  $\mu\text{m}$ . Our WSi detector integrated with Nb rails is depicted in Figure 1(a). An SEM image of a fabricated 50  $\mu\text{m}$ -wide SSPD with 4  $\mu\text{m}$ -wide adjacent Nb rails is shown in Figure 1(b). Here the Nb rails are displaced by 150 nm from the edge of the SSPD. The 3 nm-thick WSi strip has a constriction length of

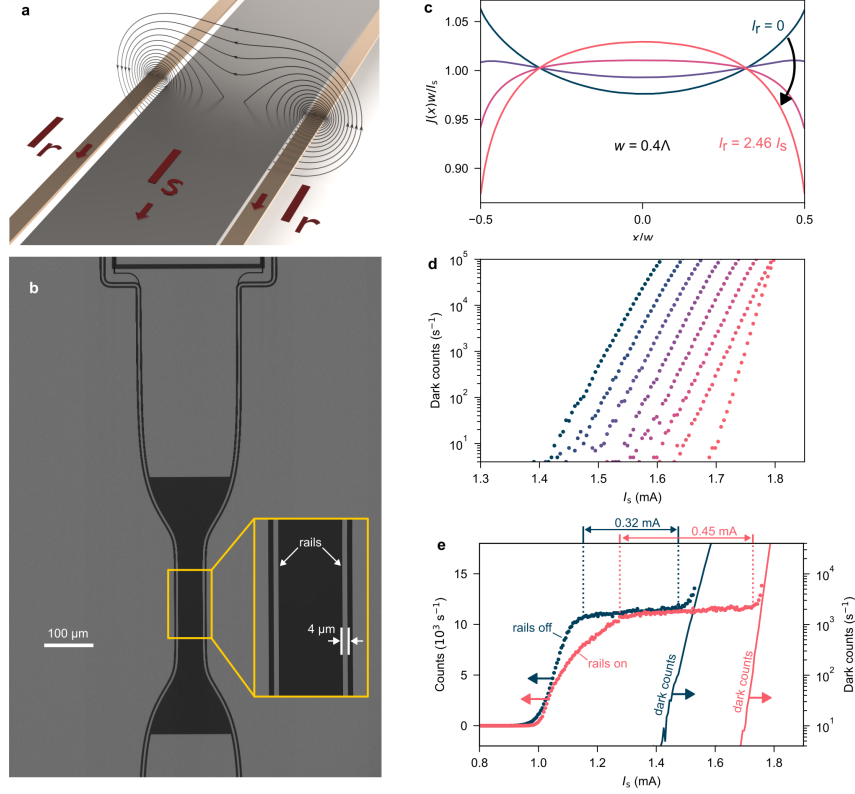

**Fig. 1** (a) Illustration of SSPD (gray) integrated with adjacent rails (gold). The rails are displaced slightly from the edge of the strip. Magnetic field lines are shown to demonstrate how the rails modify the self-induced magnetic field of the SSPD. (b) SEM image of 50  $\mu\text{m}$ -wide strip with 4  $\mu\text{m}$ -wide rails. The inset shows a zoomed-in image of the constriction. (c) Normalized current density as a function of position  $x$  along the wire width  $w$  calculated for a bare strip without rails (dark blue) and for a strip tuned by a series of increasing rail currents (purple to pink). For these simulations, the strip width is  $w = 0.4\lambda$  and the rails are displaced from the edges of the strip horizontally and vertically by  $w/200$ . (d) Measured dark count rate as a function of  $I_s$  on a 50  $\mu\text{m}$ -wide strip for a series of increasing  $I_r$  values from 0 mA (dark blue) to 13.3 mA (pink). Dark count rates onset at higher  $I_s$  as  $I_r$  is increased. (e) Measured 1550 nm photon count rate (left vertical axis, data points) and dark count rate (right vertical log-scale axis, lines) as a function of  $I_s$  for rails off (dark blue) and rails on (pink) for a 50  $\mu\text{m}$ -wide strip. Gold covers were placed over the tapers of the SSPD to prevent detection events outside the constriction, as the measurements were performed under flood illumination. The plateau width is  $\approx 320 \mu\text{A}$  with rails turned off and extends to  $\approx 450 \mu\text{A}$  with rails turned on. The start of the plateau was set as the value of  $I_s$  at which the count rate exceeds  $10.7 \times 10^3 s^{-1}$ . The end of the plateau was set as the value at which the dark count rate exceeds  $100 s^{-1}$ .

100  $\mu\text{m}$ . We have fabricated and tested numerous railed SSPDs with WSi strip widths varying from 1 to 100  $\mu\text{m}$  (see Methods). Here we present some representative results of experimental investigations of these devices.

## Suppression of dark counts

Figure 1(d) shows the dark count rate as a function of  $I_s$  for a series of  $I_r$  values for a 50  $\mu\text{m}$ -wide strip. The dark count rate follows an exponential dependence on  $I_s$ , consistent with dark counts initiated by Arrhenius thermally-activated vortex crossings. Increasing  $I_r$  from 0 mA up to 13.3 mA shifts the dark count rate curve to higher  $I_s$ . For higher values of  $I_r$  (not shown), this trend reverses and the curve shifts back to lower  $I_s$ . Here,  $I_r^* = 13.3$  mA represents the optimal rail current that maximizes the switching current  $I_{sw}$  defined at the operational dark count rate of  $100 \text{ s}^{-1}$ . At  $I_r \approx I_r^*$ , there is an abrupt increase in the slope of the dark count rate curve that persists for  $I_r > I_r^*$ . As will be discussed below, this slope increase is indicative of a transition from a regime in which dark counts are dominated by penetration of vortices from the edges ( $I_r < I_r^*$ ), to a regime in which dark counts are dominated by unbinding of vortex-antivortex (VAV) pairs in the bulk ( $I_r > I_r^*$ ).

## Rails impact on photosensitivity

Figure 1(e) shows the count rate as a function of  $I_s$  of the same 50  $\mu\text{m}$ -wide device under flood illumination of 1550 nm light with the rails off ( $I_r = 0$  mA) and with the rails on ( $I_r = I_r^*$ ). The count rate reaches a detection plateau, indicating saturated internal detection efficiency (IDE), both with the rails on and off. Note that with the rails on, the onset of photosensitivity  $I_i$  shifts to higher  $I_s$  compared to that with the rails off. However, the dark count onset shifts by an even larger amount, resulting in a nearly 40% increase in the detection plateau  $I_i < I_s < I_{sw}$ .

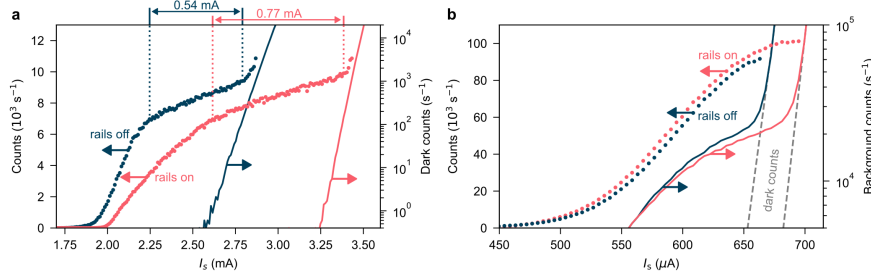

**Fig. 2** (a) Measured flood-illuminated 1550 nm photon count rate (left vertical axis, data points) or dark count rate (right vertical log-scale axis, lines) as a function of  $I_s$  for rails off (dark blue) or rails on (pink) for a 100  $\mu\text{m}$ -wide strip. The plateau width is  $\approx 540 \mu\text{A}$  with rails turned off and extends to  $\approx 770 \mu\text{A}$  with rails turned on. The start of the plateau was set as the value of  $I_s$  at which the count rate exceeds  $6.9 \times 10^3 \text{ s}^{-1}$ . The end of the plateau was set as the value at which the dark count rate exceeds  $100 \text{ s}^{-1}$ . (b) Measured flood-illuminated 4  $\mu\text{m}$  photon count rate (left vertical axis, data points) and background count rate (right vertical log-scale axis, lines) on a 20  $\mu\text{m}$ -wide strip as a function of  $I_s$  for rails off (dark blue) and rails on (pink). At low  $I_s$  the background counts are dominated by blackbody background photons entering through the free-space coupled cryostat, then, as  $I_s$  is increased, the exponential dark counts takeover as indicated by the dashed gray line. Turning on the rails shifts the dark counts to higher  $I_s$  enabling measurements at higher  $I_s$ . In this region, a rollover of counts is observed, indicating the start of a plateau and near unity IDE.

Shown in Fig 2(a) is the count rate as a function of  $I_s$  of a 100  $\mu\text{m}$ -wide device under flood illumination of 1550 nm light with the rails off ( $I_r = 0$  mA) and with the rails on ( $I_r = I_r^*$ ). The plateau in the count rate has a slope which we attribute to photon detections in the taper of the device. In contrast, the plateau in Fig. 1(e) is flat, as the tapers in that device were intentionally blocked with a gold layer. Similar to Fig. 1(e), turning the rails on shifts the onset of photosensitivity to higher  $I_s$ , while the dark-count onset shifts by a larger amount, resulting in a 43% overall increase in the detection plateau length.

We have measured the MIR photosensitivity of a 20  $\mu\text{m}$ -wide strip. For this measurement, we used a cryostat with an optical window for free-space coupled infrared light sources and a monochromator for precise wavelength selection (FIXME citation varun or ben). This optical window resulted in higher background photon counts than for measurements performed at 1550 nm [Fig. 1(d) and Fig. 2(a)]. Figure 2(b) shows the photon count rate of the 20  $\mu\text{m}$ -wide SSPD under flood illumination of 4  $\mu\text{m}$  photons as a function of  $I_s$  with the rails off and with the rails on. The background characteristic of this cryostat is evident in the  $I_s = 550$   $\mu\text{A}$  to 675  $\mu\text{A}$  range before the log-linear dark counts dominate. By turning on the rails, the dark counts are reduced enabling measurement of the 20  $\mu\text{m}$ -wide strip's photon count rate at higher  $I_s$ . The count rate at higher  $I_s$  increases and rolls over onto the start of a detection plateau, indicating a nearly 100% IDE.

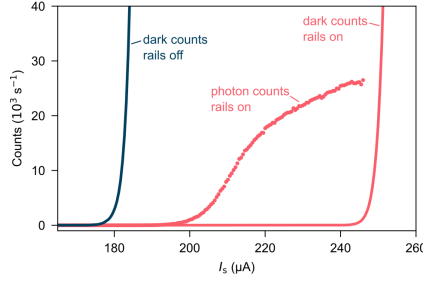

**Fig. 3** Measured flood-illuminated 1550 nm photon count rate (pink data points) and dark count rate (lines) on a low  $I_{sw}/I_d$  10  $\mu\text{m}$ -wide strip as a function of  $I_s$  for rails off (dark blue) and rails on (pink). With the rails off, the dark counts begin to dominate at such a low  $I_s$  that photon counts cannot be measured. With the rails on, a huge shift of dark counts to higher  $I_s$  is observed, and photon counts are measured with unity IDE.

We also tested several 10  $\mu\text{m}$ -wide SSPDs that showed unusually low  $I_{sw}/I_d$  ratios, which we attribute to a higher prevalence of lithographic defects in this subset of devices. In Fig. 2(b), the measured flood-illuminated 1550 nm photon count rate and dark count rate is plotted as a function of  $I_s$  for one of these devices with  $I_{sw}/I_d \approx 0.44$  in the absence of rail current. With the rails off, the dark counts dominate at such low  $I_s$  values that the strip has no photosensitivity to 1550 nm photons. With the rails on, the dark count curve shifts dramatically to higher  $I_s$ , restoring a nearly 100% IDE. Thus, the rails recovered the performance of the SSPD that otherwise would have been non-functional for 1550 nm photons.

## Rails impact on timing jitter

Figure 4(a) shows the histogram of detection latency of a 20  $\mu\text{m}$ -wide strip under 1550 nm flood illumination for six equally-spaced  $I_r$  values ranging from  $I_r = 0$  to  $I_r = 8.8$  mA. The long tail likely results from detection events in the taper of our strips, as these measurements were performed on devices without gold covers over the tapers. As  $I_r$  is increased, the histogram narrows. This may result from merging two latency distributions: one originating from edge vortex-mediated detections and another from center VAV-pair-mediated detections, but this issue requires a more thorough study.

In Fig. 4(b) the full width at half-maximum (FWHM) jitter is plotted as a function of  $I_r$  for several devices with widths ranging from 5  $\mu\text{m}$  to 20  $\mu\text{m}$ . There is no clear dependence of jitter on the strip width; however, all strips demonstrated improved jitter upon application of rail current until an optimum value is reached. At currents higher than this optimum jitter value, the jitter begins slowly increasing with the rail current. Interestingly, the optimum jitter of all three strip widths is similar,  $\approx 35$  ps. This may be due to longitudinal geometric jitter, which arises from the length of the constriction, which in this case is 300  $\mu\text{m}$ .

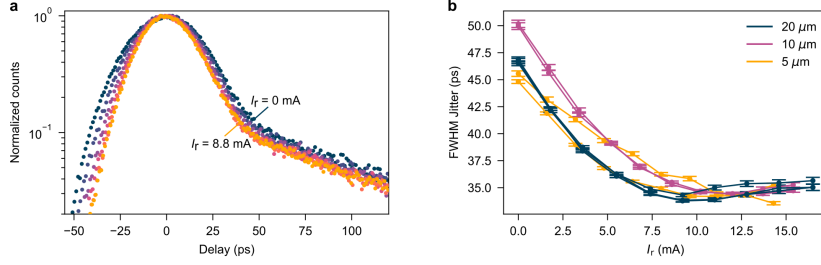

**Fig. 4** (a) Jitter histograms for a 20  $\mu\text{m}$ -wide strip under 1550 nm flood illumination for six equally-spaced  $I_r$  values ranging from  $I_r = 0$  to  $I_r = 8.8$  mA. The jitter histogram narrows as  $I_r$  is increased. (b) FWHM jitter as a function of  $I_r$  for two 5  $\mu\text{m}$  (yellow), two 10  $\mu\text{m}$  (pink) and three 20  $\mu\text{m}$  (dark blue) wide strips. As  $I_r$  is increased, the jitter decreases until it reaches a minimum.

## Increasing the switching current

As a demonstration of how the rails increase the switching current, Fig. 5 shows the ratio  $I_{sw}/I_d$  as a function of  $I_r$ . Here  $I_{sw}$  is defined as a current at which the dark count rate exceeds  $100 \text{ s}^{-1}$ . The values of  $I_d$  were obtained by measuring the change in kinetic inductance as a function of bias current in a superconducting step-impedance resonator fabricated from our WSi films (see Ref. [?] and Methods for details). For all strip widths,  $I_{sw}/I_d$  increases for positive  $I_r$  and, with the exception of the 20  $\mu\text{m}$  device, reaches a peak at  $I_r = I_r^*$  over the range of  $I_r$  measured. As the strip width increases, the change in  $I_{sw}/I_d$  becomes more significant. This trend is consistent with our calculations which show that wider strips with stronger edge current crowding benefit more from its suppression by the rails.

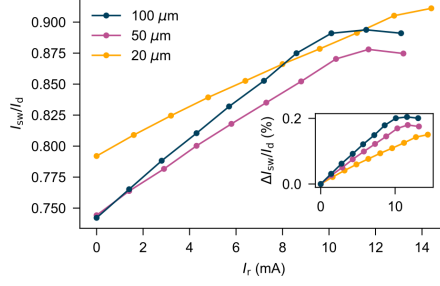

**Fig. 5** Measured  $I_{sw}/I_d$  as a function of  $I_r$  for strip widths of 20  $\mu\text{m}$  (yellow), 50  $\mu\text{m}$  (pink) and 100  $\mu\text{m}$  (dark blue). As  $I_r$  is increased,  $I_{sw}/I_d$  increases until  $I_r = I_r^*$ . Inset shows the relative change  $\Delta I_{sw}/I_d$  as a function of  $I_r$  for the same devices. As the wire width is increased, larger increases in  $I_{sw}/I_d$  were measured.

## Discussion

Our results show that integration of SSPDs with current rails reverses current crowding at the strip edges and removes the fundamental Pearl length limitation on strip width. This also follows from our numerical calculations that have shown that the current rails flatten the  $J(x)$  profile in the most part of the strip while producing controllable dips in  $J(x)$  at the edges. Moreover, the required reduction of  $J(x)$  at the edges is achieved with a normalized rail current  $I_r/I_s$  that diminishes as the strip width increases from  $w \ll \Lambda_s$  to  $w > \Lambda_s$ . We anticipate that the next limitation to scale to wider SSPD widths may be set by a degradation in film quality over large length scales.

We observed that for all devices with  $w \geq 5 \mu\text{m}$ , the switching currents reaches maxima at optimum rail currents  $I_r^*(w)$ . The slopes of the log-linear dark count rates as a function of  $I_s$  (such as that shown in Fig. 1(d)) increase abruptly at  $I_r = I_r^*$ . The dark count rate  $S$  at  $I_r < I_r^*$  generally follows a thermally-activated Arrhenius behavior caused by penetration of vortices from the edges,  $S_e(I_s) \simeq S_{e0} \exp[-(1 - I_s/I_d)U_e/T]$ , where  $U_e = \phi_0^2/2\pi\mu_0\Lambda_s \approx 61$  K sets the energy scale of the barrier for vortex entry. In turn, the nearly doubling of the logarithmic slope observed at  $I_r > I_r^*$  is a strong experimental evidence that the dark count rate becomes dominated by the unbinding of VAV pairs of radius  $\sim \xi J_d/J_s \ll w$  inside the strip. This is because the energy of a vortex spaced by  $u$  from an ideal edge of a strip is half the energy of a VAV pair of radius  $u$  inside a strip, so that now the dark count rate is given by  $S_b(I_s) \simeq S_{b0} \exp[-(1 - I_s/I_d)U_b/T]$  where  $U_b = 2U_e = \phi_0^2/\pi\mu_0\Lambda_s \approx 122$  K.

As shown in Appendix D, the ratio of the logarithmic slopes  $\partial_I \ln S$  for vortex hopping from the edges and the bulk VAV pair production are related by  $(\partial_I \ln S_b / \partial_I \ln S_e) \simeq 2\tilde{J}_d/J_d$ , where  $J_d$  and  $\tilde{J}_d$  are the mean depairing current densities in the bulk and at the edges, respectively. Here  $\tilde{J}_d$  is reduced relative to the mean  $J_d$  by the current crowding at lithographic defects. For instance, the slope ratio 1.76 observed in a 20  $\mu\text{m}$  strip implies  $\tilde{J}_d = 0.88J_d$ . To mitigate penetration of vortices from the edges for this strip, the rails should carry current sufficient to reduce  $J(x)$  at the edges by 12%, consistent with our numerical results shown in Fig. 1e.

Two important conclusions follow from our analysis of dark counts: (1) In addition to increasing  $I_{sw}$ , the rails greatly (up to 8 orders of magnitude) reduce dark counts caused by penetration of vortices from the edges. (2) At  $I_r = I_r^*$  the strip achieves its maximum depairing current fraction  $I_{sw}/I_d$  for a given dark count rate  $S_c$ . We define  $I_{sw}$  as the current at which the dark count rate reaches  $S_c = 100 \text{ s}^{-1}$ . The VAV pair unbinding makes it impossible to reach  $I_s = I_d$  in a strip without switching to the normal state, but the rails do allow the device to operate at its intrinsic performance limit at the dark count rate  $S_c$  required by a particular application. Besides the fundamental limits of  $I_{sw}$  and the SSPD sensitivity, which are both caused by the bulk VAV pair production, there are also technological and materials science limitations, resulting from variations in film thickness, lithographic defects, inhomogeneities of superconducting properties due to local non-stoichiometry, grain boundaries in polycrystalline films, film adhesion with the substrate, etc. Furthermore, our method for estimating  $I_d$  of our devices uses assumptions of the BCS model, which does not account for the effects of strong electron-phonon pairing of the Eliashberg theory (FIXME citation), or the reduction of  $J_d$  by subgap quasiparticle states (FIXME citation) which are especially pronounced in thin superconducting films. Nonetheless, tuning  $J(x)$  by rails enables reaching the operational limit of  $I_{sw}$  for a particular SSPD even if neither the exact value of  $J_d$  nor the extent of reduction of  $J_d$  at the edges is known.

We observed that current redistribution in WSi strips was possible without affecting detection efficiency uniformity; the photon count rate on the detection plateau varies by less than 1% across the full range of  $I_r$ . However, the results shown in Fig. ?? clearly show that the onset of photosensitivity shifts slightly to higher  $I_s$  with the rails on. This behavior may reflect a nonuniform threshold current density for photodetection across the strip in which the photon detections near the edge have a lower detection threshold current density than that in the bulk [? ? ?]. In this scenario, as  $I_s$  increases, the edges become photosensitive first if the rails are off. However, if the rails are turned on, the current density near the edges is reduced, so a higher total  $I_s$  is required for the edge to reach the same threshold, shifting the onset of photosensitivity to higher  $I_s$ . We also observed a broadening of the photosensitivity onset with the rails turned on. This may be consistent with a modification of the threshold current-density profile with increasing  $I_r$ . However, several mechanisms are known to influence the functional form of the internal detection efficiency as a function of bias current [? ]. Analysis of these possible mechanisms is beyond the scope of this work.

Fabrication of SSPDs inevitably produces lithographic defects at the edges of the strip. In a new fabrication process, it can be difficult to distinguish between poor fabrication quality and material performance. Our rail design can be used to effectively de-convolve fabrication quality and material performance by accessing the bulk of the film rather than being limited by the edge defects and thus to test the true performance potential of the film. This could be used as a diagnostic tool while working on improving a fabrication process until the performance without the rails is nearly that of the bulk film. Furthermore, rails can increase fabrication yield, as we demonstrated with the  $10 \mu\text{m}$ -wide strip in Fig. 2(b). This can be used to avoid tedious repeated fabrication runs and may be essential for enabling high pixel count SSPD arrays.

We would like to bring attention to the strikingly low timing jitter  $\sim 50$  ps observed on our devices up to  $20\text{ }\mu\text{m}$ -wide. These results seem inconsistent with models in which components of the VAV pair generated by a photon near the edge and in the center of the strip have different transit times [?] so that wider strips would have greater timing jitter. This model, along with previous experiments studying jitter dependence on strip width [?] have primarily focused on nanostrips  $\approx 100$  nm wide. It remains unclear how the jitter scales as the widths increase to  $1\text{-}100\text{ }\mu\text{m}$ . For instance, taking the terminal velocity of a vortex  $v_c \simeq 10\text{-}20$  km/s measured on Pb film bridges [?] at  $J_s \approx J_d$ , one would expect a jitter  $\sim w/v_c \sim 1$  ns in a  $20\text{ }\mu\text{m}$  wide strip, which is 20 times larger than the observed jitter of  $\sim 50$  ps shown in Fig. 4. The value of  $v_c$  observed on Pb is qualitatively consistent with the estimate  $v_c \simeq J_d/\eta \simeq \rho_n \xi_s / 2\mu_0 \lambda_s^2$ , where  $\eta = \phi_0^2 / 2\pi \xi_s^2 \rho_n$  is the Bardeen–Stephen vortex drag coefficient and  $J_d \simeq \phi_0 / 4\pi \mu_0 \lambda_s^2 \xi_s$ . The same estimate of  $v_c$  made for our WSi film with  $\xi_s = 10$  nm,  $\lambda_s = 950$  nm and  $\rho_n = 2.5\text{ }\mu\Omega \cdot \text{m}$  yields  $v_c \sim \rho_n \xi_s / 2\mu_0 \lambda_s^2 \sim 11$  km/s, which again predicts a jitter substantially larger than that we observed on the  $20\text{ }\mu\text{m}$  wide SSPD. Thus, real devices significantly outperform the estimates of models of vortex-assisted jitter, showing that our current understanding of the dynamics of a resistive domain produced by photon absorption is still incomplete.

It is worth noting that the ultra wide SSPDs studied here showed broad detection plateaus for  $1550$  nm photons even without applying rail current. In addition, a control device without rails, or otherwise any niobium nearby, also demonstrated a similar detection plateau, indicating that the rail structures are not required for high efficiency photosensitivity to  $1550$  nm photons. This result is remarkable, and we attribute this to two factors: (1) our fabrication process which minimized the likelihood for lithographic defects and (2) our choice of SSPD material. To the former point, our SSPDs were fabricated using electron-beam lithography and designed with relatively short strip lengths, both of which help minimize the number of edge defects (cite dependence of  $I_{sw}$  on wire length) and resulted in a fairly high  $I_{sw}/I_d$  compared to those noted in previous works (FIXME citations). To the latter point, our detector material is a highly uniform amorphous superconductor with no current-impeding grain boundaries and the thin film WSi recipe has a high silicon content ( $\approx 0.48$  Si mole fraction) designed to maximize photosensitivity in wide strips [?]. We also note that our strips do not self reset without shunting the device with an inductor and resistor in parallel with the SSPD at low temperature. This behavior is likely generic to ultra-wide SSPDs and may have caused wide strips to be overlooked in the past.

Recently Yabuno et al [?] demonstrated SSPDs of width  $20\text{ }\mu\text{m}$  ( $18\text{ }\mu\text{m}$ -wide active area). In this study, the authors used a high-critical current bank (HCCB) structure, in which the center of the strip material is irradiated with ions to selectively lower  $J_d$  relative to the edges. For a fixed current flowing through the strip, this irradiation allows the central photo-receiving region to operate at  $J_s$  closer to  $J_d$  than without irradiation. This approach demonstrated 100% IDE at  $1550$  nm for the  $20\text{ }\mu\text{m}$ -wide strip. However, the HCCB does not suppress the edge current crowding caused by the Pearl screening, but instead partially compensates for it by reducing  $J_d$  in the center relative to the edges, which would also increase dark count rate due to VAV unbinding. If the strip width approaches or exceeds  $\Lambda_s$ , the current crowding will continue to grow

and eventually exceed the additional vortex energy barrier provided by the HCCB. Therefore, the fundamental limitation on the maximum size of strip width achievable using this approach is still limited by the Pearl length.

Finally, in addition to boosting the performance limits of SSPD, the rails can also help in revealing the Berezinskii–Kosterlitz–Thouless (BKT) transition in thin films (FIXME citation). As pointed out above, the abrupt change in the logarithmic slope of the dark count rate at the optimum rail current  $I_r^*$  shown in Fig. 1(d) is a clear experimental evidence of the suppression of single-vortex penetration from the edges and a transition to the BKT unbinding of VAV pairs inside the film. Thus, using current rails can be helpful in experimental investigations of the BKT transition without the masking effects of edge-induced vortex entry.

## 2 Conclusion

We have implemented in-situ tuning of current density profiles in SSPDs using adjacent current biased superconducting rails. To our knowledge, this is the first demonstration of the SSPD architecture allowing to break the Pearl limit. We used this approach to build a set of rail-integrated SSPDs with widths up to 100  $\mu\text{m}$ , well above the previous record 20  $\mu\text{m}$ -wide SSPD FIXME [? ], and foresee no fundamental barriers to scaling up to wider strips. Our results show that rails provide numerous benefits to SSPD technology including up to 8 orders-of-magnitude reduction in dark counts, recovery of detector functionality in low performing devices, increased upper bound of wavelength sensitivity, and reaching the operational performance limits of SSPDs.

The orders-of-magnitude reduction in dark counts by rails has positive follow-on consequences for scaling these detectors into arrays in which total dark count rate is multiplied by the number of individual detectors, and thus can quickly add up to a the level of dark counts becoming detrimental to the array performance [? ]. A great reduction of dark counts in arrays of rail-integrated SSPD reverses this trend and allows developing even larger arrays.

The ability to scale to wide strips is important and previously was inaccessible. Wide strips eliminate the need to meander a detector to create a high fill factor [? ]. With a focused beam, all photons of interest can be collected onto our 100  $\mu\text{m}$ -wide detector. Scaling these wide strips up into arrays, the fill factor can be much higher than previous demonstrations [? ]. Furthermore, meandered detectors are sensitive to the polarization of light, with light polarized parallel to the straight sections of the detector being less efficiently detected. In the case of our wide detectors, all polarizations are detected with equal efficiency.

In future studies, we foresee being able to scale these detectors to widths wider than the Pearl length, which could yield high efficiency free-space coupled SSPDs – eliminating the need for lossy fiber optics. These detectors could immediately be applied to quantum information technology where loss is detrimental to the fidelity of the transmitted quantum state.

### Supplementary information.

**Acknowledgements.** This research was funded by NIST (https://ror.org/05xpvk416), University of Colorado Boulder

(<https://ror.org/02ttsq026>), and the DARPA DSO Synthetic Quantum Nanostructures program. The U.S. Government is authorized to reproduce and distribute reprints for governmental purposes notwithstanding any copyright annotation thereon. The work at ODU was supported by DARPA under grant HR0011-24-2-0386.

## Appendix A Fabrication

The chips were fabricated with 5 layers: 1 WSi layer with , 1 Nb layer, 1 Au layer and 2 dielectric (SiO<sub>2</sub>) spacer layers. First, we sputter a  $\approx 3$  nm-thick film of WSi on a 75 mm silicon wafer with 150 nm of thermal oxide. The film was capped with  $\approx 2$  nm  $\alpha$ Si to prevent oxidation. Next we patterned our strips using ZEP520A with electron-beam lithography. Then the film was etched using an inductively coupled plasma (ICP) etcher and an AR:SF<sub>6</sub> etch.

For the next layer, we pattern LOR3A + SPR660 using photolithography for the dielectric spacer layer. We sputter  $\approx 25$  nm SiO<sub>2</sub> and liftoff the resist – this layer isolates the WSi strip from the Nb rails. Then, we pattern LOR3A + SPR660 using photolithography for Nb liftoff. We then sputter  $\approx 100$  nm and lift it off. Next, we pattern our rails using ZEP520A with electron-beam lithography. The Nb is etched using the ICP etcher and an AR:SF<sub>6</sub> etch.

For the next layer, we pattern LOR3A + SPR660 using photolithography for the dielectric spacer layer. We sputter  $\approx 25$  nm SiO<sub>2</sub> and liftoff the resist – this layer isolates the Nb rails from the Au covers. Then we pattern strip covers in LOR3A + SPR660 using photolithography for Au liftoff. We evaporate  $\approx 100$  nm Au and lift it off.

## Appendix B Verification of 100 % Internal Detection Efficiency

As noted in Figure 1(e), a slope on our detection plateau was evident for detectors of all widths. We hypothesized that since our measurements were done using flood illumination, this slope may be due to detection events in the taper of our devices, which has been noted in previous studies [?] (FIXME add more citations). To test this hypothesis, we fabricated numerous devices with gold covers placed over the taper in order to block light from hitting this region. The only photosensitive region should in this case be the uncovered portion of the constriction. In Figure FIXME (a) we show an example of a 50  $\mu$ m device with a gold cover. The gold cover has a 10  $\mu$ m-long opening over the center of the constriction. The photon count rate curves for a 50  $\mu$ m-wide SSPD with a gold cover and without a gold cover are shown in Figure FIXME (b). Here the slope appears to be completely eliminated by the addition of the cover. For the 50- $\mu$ m-wide wire, the constriction was designed to be 100- $\mu$ m long, significantly longer than the 10  $\mu$ m-long opening in the gold cover. In the case of the 100  $\mu$ m-wide SSPD, the constriction was designed to be 10- $\mu$ m-long and the gap length in the gold cover remained the same. The reduction in the slope of the 100  $\mu$ m-wide SSPD was evident, but was not completely suppressed, likely due to misalignment between the Au and WSi layers. In future studies, we intend to verify that increasing the length of

the constriction of the 100  $\mu\text{m}$ -wide SSPD relative to the gap length of the gold cover suppresses the slope.

## Appendix C Depairing Current

We measured the depairing current of our film by measuring the change in kinetic inductance of the film as a function of bias current as described in Ref. [? ]. We used the reflection-mode measurement scheme and step-impedance resonators of various widths. An example of the measured change in kinetic inductance is plotted in Figure FIXME (a). From each measurement of this type, we fit the parabola to the fast and slow relaxation models and found that the fast relaxation model was a better fit. These fits were used to derive the depairing current. A summary of the measured depairing current of various resonators is shown in Figure FIXME (b). The average of these is FIXME  $\mu\text{A}$  per  $\mu\text{m}$ .

## Appendix D Field and current in the rail SSPD

Consider a long thin film strip of width  $w$  situated at  $y = 0$  between two thin film rails of width  $l$  at  $w/2 + b < x < w/2 + b + l$  and  $-w/2 - b - l < x < -w/2 - b$ , as shown in Fig. D.1. Here each rail is raised by the height  $h$  and spaced by  $b$  from the edge of the strip. It is assumed that the strip carries a dc current  $I_s$  and each rail carries a dc current  $I_r$ , both the strip and the rails are infinite along  $z$ .

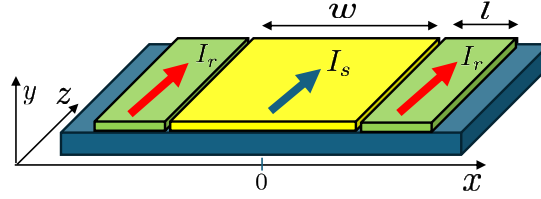

**Fig. D1** Geometry of a detector film of width  $x$  and two current rails of width  $l$ . The coordinate axes are shifted downward for clarity.

In this geometry the  $z$ -component of magnetic field  $B_z$  along the strip vanishes and other field components  $B_x = \partial A / \partial y$  and  $B_y = -\partial A / \partial x$  are expressed in terms of the  $z$  component of the vector potential  $\mathbf{A}(x, y) = [0, 0, A(x, y)]$  caused by currents flowing along  $z$ . Here  $A(x, y)$  satisfies the London equation:

$$\lambda^2 \nabla^2 A - dQ(x)\delta(y) = 0, \quad (\text{D.1})$$

where the gauge-invariant  $\mathbf{Q} = \mathbf{A} + (\phi_0/2\pi)\nabla\theta$  is proportional to the supercurrent density  $\mathbf{j} = -\mathbf{Q}/\mu_0\lambda^2$  in the film,  $\theta$  is the phase of the superconducting order parameter,  $\phi_0$  is the magnetic flux quantum,  $\lambda$  is the London penetration depth,  $d$  is the film thickness. In the planar geometry considered here  $j_x = j_y = 0$  and  $j_z(x)$  flowing along

the strip and the rails can depend only on  $x$  so the phase gradient  $\nabla\theta = (0, 0, \theta')$  has only a constant  $z$ -component  $\theta'$  independent of  $x$ . We consider here films with  $d \ll \lambda$  in the absence of vortices and  $Q \ll \phi_0/2\pi\xi$  for which the linear London electrodynamics is applicable, where  $\xi$  is a coherence length. Solution of Eq. (D.1) is given by:

$$A(x, y) = \frac{d_s w}{8\pi\lambda_s^2} \int_{-1}^1 \ln[(x-u)^2 + y^2] Q_s(u) du + \quad (D.2)$$

$$\frac{d_r w}{8\pi\lambda_r^2} \left[ \int_{1+b}^{1+b+l} \ln[(x-u)^2 + (y-h)^2] Q_r(u) du + \int_{-1-b-l}^{-1-b} \ln[(x-u)^2 + (y-h)^2] Q_r(u) du \right],$$

where  $Q_s(x)$  and  $Q_r(x)$  determine the supercurrent densities in the strip and the rails, respectively. Here  $\lambda_s$  and  $\lambda_r$  are the London penetration depths in the strip and the rail,  $d_s$  and  $d_r$  are their respective thicknesses, and all lengths are in units of  $w/2$ . Using  $Q_s(u) = Q_s(-u)$  and  $Q_r(u) = Q_r(-u)$  reduces Eq. (D.2) to

$$A(x, y) = k_s \int_0^1 \ln[((x-u)^2 + y^2)((x+u)^2 + y^2)] Q_s(u) du +$$

$$k_r \int_{1+b}^{1+b+l} \ln[((x-u)^2 + (y-h)^2)((x+u)^2 + (y-h)^2)] Q_r(u) du, \quad (D.3)$$

where  $k_s = w/4\pi\Lambda_s$ ,  $k_r = w/4\pi\Lambda_r$ , and  $\Lambda_s = 2\lambda_s^2/d_s$  and  $\Lambda_r = 2\lambda_r^2/d_r$  are the Pearl screening lengths in the strip and rails, respectively. Setting  $y = 0$  in Eq. (D.3) and using  $A(x, 0) = Q(x, 0) - \phi_0\theta'/2\pi$  gives two equations for  $Q_s(x)$  and  $Q_r(x)$ :

$$Q_s(x) - 2k_s \int_0^1 \ln|x^2 - u^2| Q_s(u) du - k_r \int_{1+l}^{1+l+b} \ln[(u^2 + h^2 - x^2)^2 + 4h^2 x^2] Q_r(u) du = \alpha, \quad (D.4)$$

$$Q_r(x) - 2k_r \int_{1+b}^{1+b+l} \ln|x^2 - u^2| Q_r(u) du - k_s \int_0^1 \ln[(u^2 + h^2 - x^2)^2 + 4h^2 x^2] Q_s(u) du = \beta, \quad (D.5)$$

where  $\alpha = \phi_0\theta'_s/2\pi$  and  $\beta = \phi_0\theta'_r/2\pi$  with constant phase gradients  $\theta'_s$  and  $\theta'_r$ .

Equations (D.4) and (D.5) were solved numerically by discretizing  $u_n = s(n-1)$ ,  $n = 1, \dots, N_1$  and introducing a vector  $Q = (Q_1, Q_2, \dots, Q_{N_1})$  which includes  $Q_s(sn)$  at  $1 < n < N$  and  $Q_r(sn)$  at  $N+1 < n < N_1$  with  $s = 1/(N-1)$ ,  $N_1 = [(1+l)N]$  and  $N = 4 \cdot 10^3$ . As a result, Eqs. (D.4) and (D.5) take the matrix form:

$$\sum_m M_{nm} Q_m = \alpha_n, \quad Q_n = \sum_m M_{nm}^{-1} \alpha_m. \quad (D.6)$$

Here  $M_{nm}$  defined by Eqs. (D.4) and (D.5) is given below,  $\alpha_n = \alpha$  at  $1 < n < N$ ,  $\alpha_n = \beta$  at  $N+1 < n < N_1$ . To express  $\alpha$  and  $\beta$  in terms of currents  $I_s = (4s/\mu_0\Lambda_s) \sum_{n=1}^N Q_n$  and  $I_r = (2s/\mu_0\Lambda_r) \sum_{n=N+1}^{N_1} Q_n$ , we sum up the second Eq. (D.6) over  $n$  using that

$\alpha_m$  are constants at  $1 < m < N$  and  $N + 1 < m < N_1$  and obtain:

$$I_s = A\alpha + B\beta, \quad I_r = A_1\beta + B_1\alpha, \quad (\text{D.7})$$

Hence,

$$\alpha = \frac{A_1 I_s - B I_r}{A A_1 - B B_1}, \quad \beta = \frac{A I_r - B_1 I_s}{A A_1 - B B_1}, \quad (\text{D.8})$$

where

$$A = \frac{4s}{\mu_0 \Lambda_s} \sum_{n=0}^N \sum_{m=0}^N M_{nm}^{-1}, \quad B = \frac{4s}{\mu_0 \Lambda_s} \sum_{n=0}^N \sum_{m=N+1}^{N_1} M_{nm}^{-1}, \quad (\text{D.9})$$

$$A_1 = \frac{2s}{\mu_0 \Lambda_r} \sum_{n=N+1}^{N_1} \sum_{m=N+1}^{N_1} M_{nm}^{-1}, \quad B_1 = \frac{2s}{\mu_0 \Lambda_r} \sum_{n=0}^N \sum_{m=N+1}^{N_1} M_{nm}^{-1} \quad (\text{D.10})$$

The matrix elements  $M_{nm}$  are given by

$$\begin{aligned} M_{nm} &= \delta_{nm} - 2k_s s \ln |(n^2 - m^2)s^2|, \quad 0 < n < N, \quad 1 < m < N, \\ M_{nm} &= -k_r s \ln [(m^2 - n^2)s^2 + h^2]^2 + (2hns)^2, \quad 0 < n < N, \quad N + 1 < m < N_1, \\ M_{nm} &= -k_s s \ln [(m^2 - n^2)s^2 + h^2]^2 + (2hns)^2, \quad N + 1 < n < N_1, \quad 1 < m < N, \\ M_{nm} &= \delta_{nm} - 2k_r s \ln |(n^2 - m^2)s^2|, \quad N + 1 < n < N_1, \quad N + 1 < m < N_1. \end{aligned}$$

The reduction of the sheet current density  $J(x) = dj(x)$  at the edges by the magnetic field produced by rails comes from off-diagonal elements of  $M_{nm}$  accounting for the inductive coupling of rails and SSPD. Examples  $J(x)$  in strips of different widths calculated from Eqs. (D.4) and (D.5) are shown in Figs. 1(a) and D2. Particularly, Fig. D2(b) shows that a nearly flat  $J(x)$  profile with the rail-controlled reduction of  $J(x)$  at the edges can be obtained in a strip 4 times wider than the Pearl length. For  $\Lambda \approx 600 \mu\text{m}$  for our WSi films, Fig. D2(b) corresponds to a 2.4 mm wide strip. After  $Q_s(x)$  and  $Q_r(x)$  have been obtained, the magnetic field around the railed SSPD is calculated using Eq. (D.2), as shown in Fig. 1(a).

## Appendix E Energy barriers and dark count rates caused by vortices

The position-dependent energy of a vortex  $E(x)$  in a thin film of width  $w \ll \Lambda_s$  calculated in the London model is given by [?]:

$$E(x) = \epsilon \ln \left( \frac{w}{\pi \xi} \sin \frac{\pi x}{w} \right) - \phi_0 J_s x, \quad (\text{E.1})$$

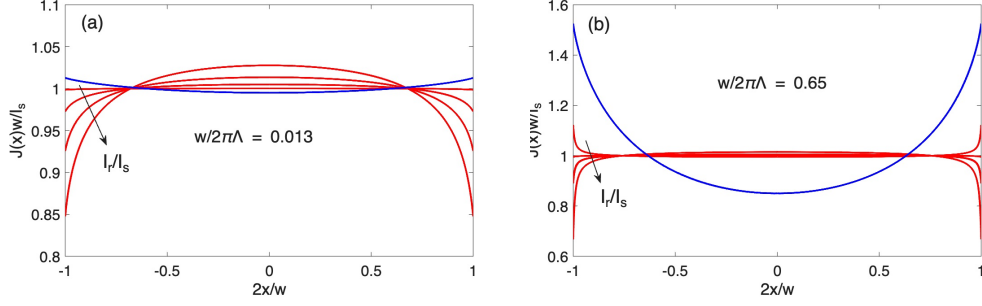

**Fig. D2** Sheet current density  $J(x)$  calculated for different film widths  $w$  and normalized rail currents  $I_r/I_s$  for the parameters of WSi films with  $d_s = 3$  nm,  $\Lambda_s = 602$   $\mu\text{m}$ ,  $k_r = 200k_s$  and  $l = 0.15w$ : (a)  $w \approx 50$   $\mu\text{m}$ ,  $I_r/I_s = 2.5, 5.03, 7.58, 10.12$ , (b)  $w \approx 2.5$  mm,  $I_r/I_s = 0.64, 0.82, 1.01, 1.21$ .

where  $\epsilon = \phi_0^2/2\pi\mu_0\Lambda_s$  is the vortex line energy, the effective  $\tilde{\xi} \approx 0.34\xi_s$  accounts for the vortex core energy, and  $J_s$  is a uniform sheet current density. The maximum in  $E(x)$  occurs at  $x = x_m$ , where:

$$x_m = \frac{w}{\pi} \cot^{-1} \frac{J_s}{J_0}, \quad J_0 = \frac{\pi\epsilon}{\phi_0 w} = \frac{\phi_0}{2\mu_0 w \Lambda_s} \sim \frac{\xi_s}{w} J_d \ll J_d \quad (\text{E.2})$$

The London model with a point vortex core is applicable for a wide strip with  $w \sim (10^2 - 10^3)\xi_s$ , but becomes invalid for a vortex spaced by  $\sim \xi_s$  from the edges. Here  $E(x)$  given by Eq. (E.1) diverges logarithmically at  $x \rightarrow 0$ , whereas the energy of a vortex emerging from the strip edge vanishes. Numerical calculations of  $E(x)$  using the Ginzburg-Landau equations [?] have shown that the London model describes  $E(x_m)$  well if  $J_s$  is not too close to  $J_d$ , and the energy barrier at  $J_s = J_d$  vanishes. To take this effect into account, we define the energy barrier for the vortex entry as  $U = E[x_m(J)] - E[x_m(J_d)]$ , where  $E(x)$  and  $x_m$  are given by Eq. (E.1) and (E.2). At  $J_s \gg J_0$  this yields the energy barrier independent of the film width:

$$U = \epsilon \ln(J_d/J_s), \quad J_s \gg J_d \xi/w. \quad (\text{E.3})$$

This gives a reasonable estimate of  $U(J)$  at  $J_s \simeq J_d$  at which  $x_m \sim \xi_s \ll w$  shifts close to the edge of the film, as depicted in Fig. E1. Thermally-activated hopping of vortices over the edge barrier results in a mean dc voltage  $V = V_0(J_s/J_d)^{\epsilon/T}$ , where  $V_0$  was evaluated in [?]. At  $\epsilon/T \gg 1$  and  $J_s \simeq J_d$  the V-I curve takes the form:

$$V = V_0 \exp[-U/T], \quad U \simeq \epsilon(1 - J_s/J_d). \quad (\text{E.4})$$

For our 3 nm thick WSi films with  $\lambda = 950$  nm and  $\Lambda = 602$   $\mu\text{m}$ , we get  $\epsilon \simeq 61$  K. At  $J_s = 0.9J_d$  and  $T = 1$  K the probability of thermally-activated penetration of a vortex from an ideal film edge is proportional to the small Arrhenius factor  $\propto \exp(-U/T) \sim 2 \cdot 10^{-3}$  which can increase substantially due to edge defects which locally reduce the energy barrier and facilitate penetration of vortices. Edge defects

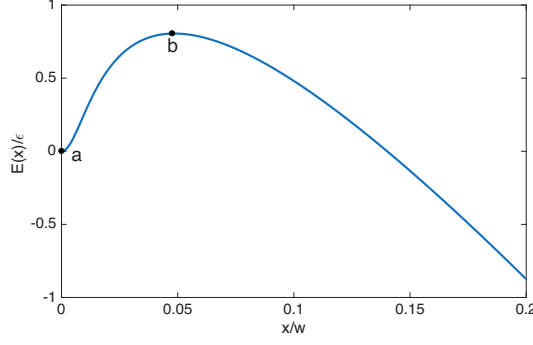

**Fig. E1** Qualitative dependence of  $E(x)$  on the vortex position evaluated from Eqs. (D.1) regularized by  $x \rightarrow \tilde{x} = [x^2 + \tilde{\xi}^2]^{1/2}$ ,  $E(x) \rightarrow E(\tilde{x}) + \phi_0 J_s \tilde{\xi}$ ,  $\tilde{\xi} = 10^{-2}w$  and  $J_s = 20J_0$ .

can be small indentations or other microstructural features causing local variations of  $T_c$  or current crowding around defects. For instance, the local current density at the edge of a semicircular indentation of radius  $R \gg \xi$  is twice the mean  $J_s$ , and larger concentration of impurities at the edges causes local reduction of  $J_d$ . Such defects serve as gates for local penetration of vortices for which the energy barrier  $U(J_s)$  vanishes at the mean current density  $\tilde{J}_d$  smaller than the bulk  $J_d$ . Given many material uncertainties depending on the film growth and deposition parameters, we assume that edge imperfections locally reduce the mean depairing density to  $\tilde{J}_d < J_d$  in a narrow strip along the edges. It is the reduction of  $\tilde{J}_d$  at the edge which is mitigated by the current rails. With that in mind, consider now the number  $S_e$  of thermally-activated vortices penetrating over the edge barrier per unit time in a film of length  $L$ :

$$S_e = S_{e0} \exp \left[ -\frac{\epsilon}{T} \left( 1 - \frac{J_s}{\tilde{J}_d} \right) \right], \quad S_{e0} \sim \frac{L\nu}{l_i} \quad (\text{E.5})$$

Here  $L/l_i$  is a number of statistically-independent vortex entries through edge defects with a mean spacing  $l_i$  and  $\nu$  is an attempt frequency. In the overdamped limit characteristic of Abrikosov vortices,  $\nu \simeq \sqrt{k_a k_b} / 4\pi\eta$  follows from the classical result of Kramers [?], where  $k_a$  and  $k_b$  are curvatures of  $E(x)$  at the bottom and the top of the potential well depicted in Fig. E1,  $\eta = \phi_0^2 d_s / 2\pi \xi^2 \rho_n$  is the Mattis-Bardeen vortex drag coefficient, and  $\rho_n$  is the normal state resistivity. Taking  $\sqrt{k_a k_b} \sim \phi_0^2 d_s / 4\pi \mu_0 \lambda_s^2 \xi_s^2$  at  $J_s \sim \tilde{J}_d$  in Eq. (E.5) yields

$$S_{e0} \sim \frac{L\rho_n}{8\pi\mu_0\lambda_s^2 l_i} \quad (\text{E.6})$$

For a WSi film with  $L = 0.1$  mm,  $\lambda = 950$  nm,  $\rho_n = 2.5 \mu\Omega\text{m}$  and  $l_i \sim 10^2$  nm, we get  $S_{e0} \sim 10^{12} \text{ s}^{-1}$ . Here Eq. (D.6) is a rough, order of magnitude estimate which takes into account neither microstructural details of edge imperfections nor deformation of the vortex core at the edge in the presence of current [?]. The latter can result an extra factor  $(1 - J_s/J_d)^n$  with  $n = 1 - 2$ , yet the logarithmic slope

$$\frac{d \ln S_e}{d J_s} = \frac{\epsilon}{T \tilde{J}_d} \quad (\text{E.7})$$

is practically insensitive to uncertainties in  $S_{e0}$  and its possible power-law dependence on  $J_s$  if  $T \ll \epsilon$ .

From Eq. (E.5), we obtain a maximum current  $I_{c1}$  which SSPD can carry at a given dark count rate  $S_c$ :

$$I_{c1} = \tilde{I}_d \left( 1 - \frac{T}{\epsilon} \ln \frac{S_{e0}}{S_c} \right) \quad (\text{E.8})$$

For  $S_c = 10^2 \text{ s}^{-1}$  used in our definition of  $I_{sw}$ ,  $S_{e0} = 10^{12} \text{ s}^{-1}$  and  $T/\epsilon = 1/61$  at 1 K, we get  $I_{c1} \approx 0.62 \tilde{I}_d$ , where  $\tilde{I}_d = w \tilde{J}_d$ . Such operational  $I_{c1}$  equivalent to  $I_{sw}$  is limited by the acceptable dark count rate  $S_c$  and decreases logarithmically with the SSPD length. The account of the extra factor  $(1 - J_s/\tilde{J}_d)$  in  $S_{e0}$  only increases  $I_{c1}$  by 3% and is neglected hereafter.

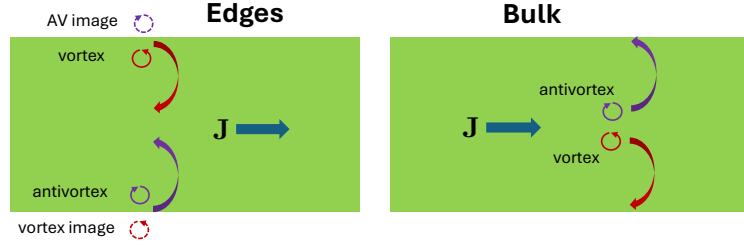

**Fig. E2** Single vortices and antivortices penetrating from the film edges and vortex-antivortex pair unbinding inside the film due to thermal fluctuations.

Consider now the critical current  $I_{c2}$  limited by thermally-activated unbinding of VAV pairs inside the film. This process is illustrated in Fig. E2, from which it follows that the energy scale for the VAV pair production is twice that of the vortices penetrating from the edges:

$$U = 2\epsilon \left( 1 - \frac{J_s}{J_d} \right), \quad J_s \sim J_d \quad (\text{E.9})$$

This barrier vanishes at the bulk  $J_d$  larger than  $\tilde{J}_c$  for penetration of vortices from the edges. The VAV production rate in a film at  $J_s \sim J_d$  can be evaluated in the same way as it was done above:

$$S_b = S_{b0} \exp \left[ -\frac{2\epsilon}{T} \left( 1 - \frac{J_s}{J_d} \right) \right], \quad S_{b0} \sim \frac{A\nu}{2\pi\xi_s^2}. \quad (\text{E.10})$$

Here  $A/2\pi\xi_s^2$  is a number of statistically-independent positions of the vortex core of size  $\xi_s$  in a film of area  $A$  and

$$S_{b0} \sim \frac{A\rho_n}{16\pi^2\mu_0\lambda_s^2\xi_s^2}. \quad (\text{E.11})$$

The critical current limited by the bulk VAV pair production is then

$$I_{c2} = I_d \left( 1 - \frac{T}{2\epsilon} \ln \frac{S_{b0}}{S_c} \right) \quad (\text{E.12})$$

For  $A = 20 \mu\text{m} \times 100 \mu\text{m}$ ,  $\rho_n = 2.5 \mu\Omega\text{m}$ ,  $\lambda_s = 950 \text{ nm}$ ,  $\xi_s = 10 \text{ nm}$  and  $T/2\epsilon = 1/122$ , Eqs. (E.11) and (E.12) give  $S_{b0} \sim 3 \cdot 10^{17} \text{ s}^{-1}$  and  $I_{c2} \approx 0.71 I_d$  at  $S_c = 10^2 \text{ s}^{-1}$ . Here  $I_{c2}$  limited by the bulk VAV unbinding decreases logarithmically with the SSPD area.

As follows from Eqs. (E.7) and (E.12), the logarithmic slopes of dark count rates for the VAV pair unbinding and the vortex hopping from the edges are related by:

$$\frac{d \ln S_b}{dI} = \left( \frac{2\tilde{J}_d}{J_d} \right) \frac{d \ln S_e}{dI}. \quad (\text{E.13})$$

According to our experimental data shown in Fig. 1(d), the slope  $d \ln S/dI$  abruptly increases by a factor 1.76 above a threshold current in the rails. This indicates switching from the dark counts limited by penetration of vortices from the edges to the bulk VAV pair unbinding. In this case Eq. (E.13) can be used to evaluate the extent by which lithographic defects reduce the mean depairing current density at the edges:  $\tilde{J}_d = 0.88 J_d$ . Such relatively small decrease in  $\tilde{J}_d$  is in line with the magnitude of reduction of  $J(x)$  at the edges obtained in our numerical results shown in Fig. D2(a).
